# Supplementary material for: Eliminating Delocalization Error through Localized Orbital Scaling Correction with Orbital Relaxation from Linear Response
Source: arXiv:2602.11003 ancillary file (2026-07-13)
Supplement: Supplementary file 1 [file SI.pdf]

# Eliminating Delocalization Error through Localized Orbital Scaling Correction with Orbital Relaxation from Linear Response

Yichen Fan<sup>¶,†</sup> Jincheng Yu<sup>¶,†</sup> Jiayi Du,<sup>†</sup> and Weitao Yang<sup>\*,†,‡</sup>

<sup>†</sup>*Department of Chemistry, Duke University, Durham, NC 27708*

<sup>‡</sup>*Department of Physics, Duke University, Durham, NC 27708*

E-mail: weitao.yang@duke.edu

<sup>¶</sup>These authors contributed equally.

## Resolution of the Identity like Approximation Utilizing the Sherman-Morrison-Woodbury Formula

The primary computational challenge in lrLOSC is evaluating the curvature matrix  $\kappa$ , which requires the inversion of the matrix  $M$ . As stated in the main text,  $M$  is defined as:

$$M_{ia\tau,jb\nu} = (\epsilon_{a\tau} - \epsilon_{i\tau})\delta_{ij}\delta_{ab}\delta_{\tau\nu} + n_{j\nu}(K_{ia\tau,jb\nu} + K_{ia\tau,bj\nu}), \quad (1)$$

where  $\epsilon_{i\tau}$  and  $\epsilon_{a\tau}$  are orbital energies,  $n_{j\nu}$  are occupation numbers, and  $K$  represents the Hartree-exchange-correlation kernel.

The matrix inversion, which scales as  $\mathcal{O}(N^6)$  for  $N$  electrons, poses a bottleneck for large systems. To alleviate this computational cost, we employ the Sherman-Morrison-Woodbury

(SMW)<sup>1</sup> formula alongside a Resolution-of-the-Identity (RI)<sup>2</sup> approximation to capture the orbital relaxation effect in the curvature matrix.

Following the RI-V scheme provided by Ren et al.<sup>2</sup>, the pair products of basis functions  $\rho_{ia}(\mathbf{r})$  are approximated by the auxiliary basis function  $\{f_P(\mathbf{r})\}$ , and

$$\rho_{ia}(\mathbf{r}) = \varphi_i(\mathbf{r})\varphi_j(\mathbf{r}) \approx \sum_P C_{ia}^P f_P(\mathbf{r}), \quad (2)$$

where the expansion coefficients are chosen as:

$$C_{ia}^Q = \sum_P (ia|P) V_{PQ}^{-1}, \quad (3)$$

where

$$(ia|P) = \iint d\mathbf{r} d\mathbf{r}' \frac{\rho_{ia}(\mathbf{r}) P(\mathbf{r}')}{|\mathbf{r} - \mathbf{r}'|}, \quad (4)$$

and

$$V_{PQ} = \iint d\mathbf{r} d\mathbf{r}' \frac{P(\mathbf{r}) Q(\mathbf{r}')}{|\mathbf{r} - \mathbf{r}'|}. \quad (5)$$

These approximated coefficients enable the following decomposition of the four-center ERI integral:

$$(ia|jb) = \iint d\mathbf{r} d\mathbf{r}' \frac{\rho_{ia}(\mathbf{r}) \rho_{jb}(\mathbf{r}')}{|\mathbf{r} - \mathbf{r}'|} \approx \sum_{PQ} C_{ia}^P V_{PQ}^{-1} C_{jb}^Q. \quad (6)$$

In this work, in addition to the four-center ERI integral, the interaction kernel  $K_{ia,jb}$  also includes the contribution from the exchange-correction kernel, where  $K$  is defined as:

$$K^{\tau,\nu}(\mathbf{r}_1, \mathbf{r}_2; \mathbf{r}_3, \mathbf{r}_4) = \frac{\delta(\mathbf{r}_1, \mathbf{r}_2) \delta(\mathbf{r}_3, \mathbf{r}_4)}{|\mathbf{r}_1 - \mathbf{r}_3|} + \frac{\delta^2 E_{\text{xc}}}{\delta \rho_s^\tau(\mathbf{r}_2, \mathbf{r}_1) \delta \rho_s^\nu(\mathbf{r}_3, \mathbf{r}_4)}, \quad (7)$$

and the corresponding matrix is given as:

$$K_{ia\tau,jb\nu} = (ia|jb) + \langle ia\tau | f_{\text{xc}} | jb\nu \rangle. \quad (8)$$

Analogous to the decomposition stated in Equation 6, matrix  $K$  has the following decomposition:

$$K_{ia\tau,jb\nu} = \iint d\mathbf{r}d\mathbf{r}' \frac{\rho_{ia}(\mathbf{r})\rho_{jb}(\mathbf{r}')}{|\mathbf{r} - \mathbf{r}'|} + \rho_{ia}(\mathbf{r})f_{xc}^{\tau\nu}\rho_{jb}(\mathbf{r}') \approx \sum_{PQRS} C_{ia}^P V_{PQ}^{-1} (V_{QR} + f_{QR}^{xc}) V_{RS}^{-1} C_{jb}^S. \quad (9)$$

Equation 9 circumvents the direct integration of the four-center integrals and replaces it by the product of two-center and three-center integrals.

With the RI decomposition, the matrix  $M$  can be written as:

$$M = A + X \cdot Y^T, \quad (10)$$

where:

$$A = (\epsilon_{a\tau} - \epsilon_{i\tau})\delta_{ij}\delta_{ab}\delta_{\tau\nu}, \quad X = \sum_P C_{ia}^P V_{PQ}^{-1}, \quad Y^T = \sum_{QR} (V_{QR} + f_{QR}^{xc}) V_{RS}^{-1} C_{jb}^S. \quad (11)$$

The SMW formula allows the inversion of  $M$  to be efficiently computed as:

$$M^{-1} = A^{-1} - A^{-1}X \left( I + Y^T A^{-1}X \right)^{-1} Y^T A^{-1}. \quad (12)$$

Here,  $A^{-1}$  is diagonal and easily computable, while the term  $I + Y^T A^{-1}X$  has reduced dimensions  $N_{\text{aux}} \times N_{\text{aux}}$ , making its inversion computationally efficient.

To simplify further, the diagonal matrix  $A^{-1}$  is absorbed into the matrix  $X$ :

$$\tilde{X}_{ia}^P = A_{ia}^{-1} X_{ia}^P = (\epsilon_i - \epsilon_a)^{-1} X_{ia}^P. \quad (13)$$

The resulting curvature matrix is expressed as:

$$\langle ia | M^{-1} | jb \rangle = \left[ \delta_{ia,jb} - \tilde{X}_{ia}^P \left( \delta_{PQ} + Y_{jb}^P \tilde{X}_{jb}^Q \right)^{-1} Y_{ia}^Q \right] A_{ia,ia}^{-1}. \quad (14)$$

Utilizing the SMW formula can significantly decrease computational time. However, explicitly storing and manipulating the four-center matrix can lead to a substantial memory cost, particularly for large systems. To address this challenge, a preferred strategy is circumventing any direct interaction with the  $M^{-1}$ .

In lrLOSC, the curvature is given as

$$\kappa_{pq}^{\sigma} = K_{pp\sigma,qq\sigma} - \sum_{ia\tau,jb\nu} (K_{pp\sigma,ia\tau} + K_{pp\sigma,ai\tau}) M_{ia\tau,jb\nu}^{-1} K_{jb\nu,qq\sigma}, \quad (15)$$

where  $K_{pp\sigma,qq\sigma}$  denotes the unscreened interaction, and the latter term captures the screening effect. The product  $M_{ia\tau,jb\nu}^{-1} K_{jb\nu,qq\sigma}$  is thus evaluated efficiently without explicitly forming  $M^{-1}$ , while the use of the SMW formula ensures computational scaling of  $\mathcal{O}(N^3)$  for inversion-related operations.

This method facilitates the efficient and memory-efficient computation of  $\kappa_{pq}^{\sigma}$  in lrLOSC, rendering it suitable for molecular systems of varying sizes. In the subsequent text, we plan to introduce some numerical validation tests for the RI-like SMW approach.

## Hardware and Software Details

The lrLOSC computations were performed on a high-performance computing node equipped with an Intel Xeon Gold 6226R CPU running at 2.90 GHz with 192 GB of DDR4 RAM. The GPU used was an NVIDIA A100 PCIe Tensor Core GPU with 40 GB of memory, optimized for parallel computations. The operating system was Debian GNU/Linux 12.5 (Bookworm), and the CUDA version was 12.4. The code was implemented in C with GPU kernels compiled using the NVIDIA CUDA Compiler (NVCC) targeting the `sm_80` architecture, while the host code was compiled using the Intel OneAPI C Compiler (ICC) version 2022. These specifications ensure efficient utilization of the GPU’s computational capabilities and host-side optimizations for large-scale curvature matrix evaluations.

# Time Cost and Numerical Accuracy for the RI-like SMW Approach

Building on a thorough comprehension of the computational efficiencies achieved by the RI-like SMW approximation, a study on time scaling and numerical accuracy was conducted. The molecule of interest is the all-trans polyacetylene ( $\text{H}(\text{HC}=\text{CH})_n\text{H}$ ), employing cc-pVTZ<sup>3</sup> for all computations, and cc-pVTZ-RIFIT<sup>4</sup> for the auxiliary basis set. Time consumption for the post-SCF method and the ionization potential (obtained as the negative HOMO energy) from two implementations are presented. For a direct evaluation of the RI-like SMW method’s performance, the time taken for orbital localization is excluded in both implementations.

Table 1: Comparison of computational time and ionization potential (IP) values for polyacetylene chains  $\text{H}(\text{HC}=\text{CH})_n\text{H}$  with increasing chain length ( $n$ ). Results are shown for two approaches: the SMW based RI approximation and the direct evaluation of  $M^{-1}$ . The number of electrons ( $N_{\text{Elec}}$ ) and contracted Gaussian-type orbitals ( $N_{\text{CGTO}}$ ) are also provided. “OOM” indicates an out-of-memory error, which occurs for direct  $M^{-1}$  evaluation in larger systems. The times are in unit of second and the IPs are in unit of electron-volt (eV).

| Poly acetylene $\text{H}(\text{HC}=\text{CH})_n\text{H}$ |                   |                   | SMW based RI      |         | Evaluate $M^{-1}$ directly |         |
|----------------------------------------------------------|-------------------|-------------------|-------------------|---------|----------------------------|---------|
| n                                                        | $N_{\text{Elec}}$ | $N_{\text{CGTO}}$ | post-SCF Time (s) | IP (eV) | post-SCF Time (s)          | IP (eV) |
| 1                                                        | 16                | 130               | 13.59             | 10.648  | 11.95                      | 10.639  |
| 2                                                        | 30                | 230               | 30.90             | 9.272   | 134.73                     | 9.260   |
| 3                                                        | 44                | 330               | 57.67             | 8.456   | 803.97                     | 8.446   |
| 4                                                        | 58                | 430               | 97.60             | 7.962   | 3125.41                    | 7.946   |
| 5                                                        | 72                | 530               | 157.00            | 7.430   | 9167.28                    | 7.412   |
| 6                                                        | 86                | 630               | 243.75            | 7.199   | 22803.42                   | 7.189   |
| 7                                                        | 100               | 730               | 355.24            | 6.945   | 48331.90                   | 6.938   |
| 8                                                        | 114               | 830               | 533.19            | 6.863   | OOM                        | OOM     |
| 9                                                        | 128               | 930               | 747.44            | 6.589   | OOM                        | OOM     |
| 10                                                       | 142               | 1030              | 1133.22           | 6.507   | OOM                        | OOM     |

# Evaluation of Functional Derivatives at Fractional Electron

The unstable curvature region identified by Li and coworkers<sup>5</sup> can severely affect the curvature matrix calculations in the main text, potentially leading to catastrophic numerical instability. To address this issue, a robust approach is required to avoid unstable curvatures while preserving the behavior of all other states.

In this work, we evaluate the functional derivative of the exchange-correlation ( $E_{\text{xc}}$ ) functional at fractional electron densities to bypass the unstable curvature region. Based on the Kohn-Sham (KS) energy functional:<sup>6</sup>

$$E[\rho] = T_s[\rho] + J[\rho] + E_{\text{xc}}[\rho] + \int d\mathbf{r} \rho(\mathbf{r})v(\mathbf{r}), \quad (16)$$

where  $T_s[\rho]$  is the non-interacting kinetic energy,  $J[\rho]$  is the Coulomb energy, and  $\int d\mathbf{r} \rho(\mathbf{r})v(\mathbf{r})$  is the external potential energy, the energy functional depends critically on  $E_{\text{xc}}[\rho]$ , the exchange-correlation contribution.

In the context of lrLOSC, evaluating the curvature matrix involves calculating the second functional derivative of the exchange-correlation functional with respect to the electron density:

$$f_{\text{xc}}(\mathbf{r}, \mathbf{r}') = \frac{\delta^2 E_{\text{xc}}[\rho]}{\delta \rho(\mathbf{r}) \delta \rho(\mathbf{r}')}. \quad (17)$$

This second-order functional derivative is also widely used in time-dependent density functional theory (TD-DFT). However,  $f_{\text{xc}}(\mathbf{r}, \mathbf{r}')$  can exhibit singularities, which are the root cause of the unstable curvature.

To mitigate these singularities, we introduce a modified electron density  $\rho_m$  as:

$$\rho_m = \epsilon |\psi|^2 + \rho = \epsilon |\psi|^2 + \sum_{i \in \text{occ}} n_i |\psi_i|^2, \quad (18)$$

where  $\rho$  is the original electron density obtained from the self-consistent field (SCF) calculation,  $\psi$  is the wavefunction of the molecular orbital under consideration,  $n_i$  represents the occupation number of orbital  $i$ , and  $\epsilon$  is a small positive parameter introduced to stabilize the curvature. Our numerical tests show that a small  $\epsilon$  restores stability in  $f_{xc}$  without significantly affecting other orbitals.

In order to validate the modified electron density method, in Tables I and II, we present the GSC2<sup>7</sup> corrected photoemission spectrum for water (H<sub>2</sub>O) and chlorine (Cl<sub>2</sub>), and aug-cc-pVTZ served as the MO basis set. All energy peaks were obtained via Equation (6) and Equation (7) in the main text, and the unitary operator is set to identity to remove the effect from orbital localization. The  $\epsilon = 0.03$  was applied to eliminate singularities in the exchange-correlation kernel, and the uncorrected eigenvalues were included for better comparison as well.

Table 2: Low-lying orbital energies (in eV) for H<sub>2</sub>O evaluated with and without the modified electron density.

| Orbital                | $\epsilon_{\text{uncorrected}}^{\text{BLYP}}$ | $\epsilon = 0$ | $\epsilon = 0.03$ |
|------------------------|-----------------------------------------------|----------------|-------------------|
| 2A <sub>1</sub>        | -25.224819                                    | -31.153686     | -31.149774        |
| 1B <sub>2</sub>        | -13.120699                                    | -18.611919     | -18.604761        |
| 3A <sub>2</sub>        | -9.2803073                                    | -14.581547     | -14.572619        |
| 1B <sub>1</sub> (HOMO) | -7.2100426                                    | -12.40723      | -12.401892        |
| 4A <sub>1</sub> (LUMO) | -1.0647328                                    | -3.6259013     | 0.87194426        |
| 2B <sub>2</sub>        | -0.2998129                                    | -213.48594     | 0.77025936        |

Table 3: Low-lying orbital energies (in eV) for Cl<sub>2</sub> evaluated with and without the modified electron density.

| Orbital             | $\epsilon_{\text{uncorrected}}^{\text{BLYP}}$ | $\epsilon = 0$ | $\epsilon = 0.03$ |
|---------------------|-----------------------------------------------|----------------|-------------------|
| 4 $\Sigma_g$        | -22.9500099                                   | -27.28539476   | -27.28650424      |
| 4 $\Sigma_u$        | -19.1115215                                   | -23.22572452   | -23.22721367      |
| 5 $\Sigma_g$        | -11.68228487                                  | -15.67826491   | -15.68306056      |
| 2 $\Pi_u$           | -9.66907551                                   | -13.51914123   | -13.52195771      |
| 2 $\Pi_g$ (HOMO)    | -7.27814734                                   | -11.09007295   | -11.09284708      |
| 5 $\Sigma_u$ (LUMO) | -4.53884351                                   | -0.84466223    | -0.83150927       |

For water (H<sub>2</sub>O), the orbital energy differences between the different  $\epsilon$  are negligible (less than 0.01 eV which is magnitude smaller than the MAE of lrLOSC) for all occupied orbitals.

However, significant singularities are encountered in the LUMO and LUMO+1 calculations, which are successfully mitigated by the modified density. For chlorine ( $\text{Cl}_2$ ), the LUMO calculation does not exhibit singularities, and the modified electron density maintains good agreement with the regular calculations.

## Computation details

As stated in the main text, the test set employed in this study consists of four subsets. For all the results presented in this document and in the main text, the SCF calculations for the parent DFT are carried out using Gaussian 16,<sup>8</sup> and the GSC2, LOSC2, and lrLOSC corrections are computed in a post-SCF manner using the QM<sup>4</sup>D<sup>9</sup> package. All calculation results reported in the following sections are based on PBE<sup>10</sup> parent DFT calculation. The  $\Delta$ SCF calculations adapted the Maximum Overlap Method<sup>11</sup> implemented in PySCF.<sup>12</sup>

### **Small molecules Test set (No more than 8 atoms)**

The small molecule test set includes 53 Ionization Potential (IP) and 43 Electron Affinity (EA) calculations. The test molecules are sourced from the G2/97 set,<sup>13</sup> and the reference IP and EA values are obtained from CCSD(T) calculations, extrapolated to the complete basis set limit as detailed in Ref Su et al.<sup>14</sup>. For the small molecule test set calculations, the augmented correlation consistent triple zeta (aug-cc- pVTZ)<sup>3</sup> basis set is employed. In these calculations, curvature and integrals are evaluated directly, without using the RI approximation or Sherman-Morrison’s formula.

Table 4: Comparison of vertical ionization potential (IP) values (in eV) for a set of small molecules using different methods: lrLOSC, GSC2, LOSE, and  $\Delta$ PBE. Reference values, unless specified otherwise, are obtained from CCSD(T)/aug-cc-pVTZ calculations.<sup>14</sup> The first IP is determined as the negative value of the highest occupied molecular orbital (HOMO) energy. ‘N/A’ in the  $\Delta$ PBE column indicates convergence failure for the (N-1)-electron system in self-consistent calculations. Mean absolute error (MAE) and mean signed error (MSE) are reported for each method compared to the reference.

| Molecule                      | ref   | lrLOSC (this work) | GSC2  | LOSE  | $\Delta$ PBE |
|-------------------------------|-------|--------------------|-------|-------|--------------|
| H <sub>4</sub> C              | 14.40 | 14.08              | 14.02 | 13.81 | 13.92        |
| H <sub>3</sub> N              | 11.03 | 10.91              | 10.88 | 11.47 | 11.01        |
| HO                            | 13.07 | 13.00              | 13.00 | 13.55 | N/A          |
| H <sub>2</sub> O              | 12.74 | 12.54              | 12.54 | 13.28 | 12.76        |
| HF                            | 16.20 | 15.97              | 15.97 | 16.81 | 16.25        |
| H <sub>4</sub> Si             | 12.84 | 12.45              | 12.32 | 12.06 | 12.11        |
| HP                            | 10.18 | 10.18              | 10.15 | 9.66  | 10.23        |
| H <sub>2</sub> P              | 9.82  | 9.96               | 9.91  | 9.51  | 9.96         |
| H <sub>3</sub> P              | 10.61 | 10.49              | 10.46 | 10.20 | 10.47        |
| HS                            | 10.41 | 9.96               | 10.29 | 10.03 | N/A          |
| H <sub>2</sub> S              | 10.48 | 10.33              | 10.30 | 10.08 | 10.36        |
| HCl                           | 12.82 | 12.62              | 12.61 | 12.32 | 12.69        |
| H <sub>2</sub> C <sub>2</sub> | 11.51 | 11.32              | 11.31 | 11.15 | 11.39        |
| H <sub>4</sub> C <sub>2</sub> | 10.74 | 10.63              | 10.61 | 10.49 | 10.65        |
| CO                            | 14.08 | 13.92              | 13.89 | 13.95 | 13.86        |
| N <sub>2</sub>                | 15.61 | 15.23              | 15.22 | 14.51 | 15.37        |
| O <sub>2</sub>                | 12.49 | 12.37              | 12.37 | 11.49 | 12.58        |
| P <sub>2</sub>                | 10.82 | 10.45              | 10.44 | 9.91  | 10.47        |
| S <sub>2</sub>                | 9.56  | 9.48               | 9.46  | 8.58  | 9.52         |
| Cl <sub>2</sub>               | 11.77 | 11.21              | 11.20 | 10.27 | 11.24        |
| FCI                           | 12.95 | 12.43              | 12.40 | 11.62 | 12.48        |
| CS                            | 11.51 | 11.41              | 11.38 | 11.76 | 11.31        |
| BF <sub>3</sub>               | 16.18 | 15.72              | 14.37 | 16.52 | 14.42        |
| BCl <sub>3</sub>              | 11.91 | 11.66              | 10.78 | 11.82 | 10.76        |
| CO <sub>2</sub>               | 13.90 | 13.58              | 13.58 | 12.66 | 13.63        |
| CF <sub>2</sub>               | 12.40 | 11.87              | 11.84 | 11.58 | 11.88        |
| COS                           | 11.36 | 11.22              | 11.19 | 10.60 | N/A          |
| CS <sub>2</sub>               | 10.18 | 10.01              | 10.00 | 9.14  | 10.00        |
| H <sub>2</sub> C              | 10.40 | 10.41              | 10.37 | 10.30 | 10.57        |
| H <sub>3</sub> C              | 9.78  | 9.94               | 9.88  | 9.89  | 10.01        |
| CN                            | 14.22 | 14.15              | 14.15 | 13.90 | 14.71        |
| HCO                           | 9.37  | 9.40               | 9.36  | 8.59  | 9.54         |
| CH <sub>2</sub> OH            | 8.18  | 8.11               | 8.06  | 7.73  | 8.19         |
| CH <sub>3</sub> O             | 10.94 | 10.57              | 10.52 | 10.93 | N/A          |
| H <sub>4</sub> CO             | 11.17 | 10.76              | 10.69 | 11.03 | 10.70        |

Table 5: The first IP for small molecules (continue)

| Molecule                               | ref                | lrLOSC (this work) | GSC2  | LOSC2 | $\Delta$ PBE |
|----------------------------------------|--------------------|--------------------|-------|-------|--------------|
| H <sub>3</sub> CF                      | 13.47              | 12.72              | 12.67 | 12.33 | 12.66        |
| H <sub>2</sub> CS                      | 9.47               | 9.24               | 9.21  | 8.99  | 9.24         |
| CH <sub>2</sub> SH                     | 7.79               | 7.75               | 7.70  | 7.33  | 7.75         |
| H <sub>3</sub> CCl                     | 11.49              | 11.21              | 11.13 | 10.99 | 11.10        |
| H <sub>3</sub> COF                     | 11.68              | 10.99              | 10.96 | 10.89 | 10.95        |
| C <sub>2</sub> N <sub>2</sub>          | 13.59              | 13.46              | 12.99 | 13.62 | 13.03        |
| H <sub>4</sub> B <sub>2</sub>          | 10.17              | 10.09              | 10.06 | 10.02 | 10.08        |
| HN                                     | 13.48              | 13.53              | 13.52 | 13.55 | 13.77        |
| H <sub>2</sub> N                       | 12.12              | 12.15              | 12.13 | 12.59 | 12.90        |
| H <sub>2</sub> N <sub>2</sub>          | 10.28              | 9.90               | 9.87  | 9.26  | 10.02        |
| H <sub>3</sub> N <sub>2</sub>          | 8.34               | 8.34               | 8.31  | 7.96  | 8.47         |
| HOF                                    | 13.03              | 12.43              | 12.41 | 12.02 | 12.57        |
| H <sub>2</sub> Si                      | 9.55               | 9.36               | 9.33  | 8.90  | 9.35         |
| H <sub>3</sub> Si                      | 8.86               | 8.99               | 8.93  | 8.59  | 8.92         |
| H <sub>2</sub> Si <sub>2</sub>         | 8.22               | 8.03               | 7.96  | 7.58  | 7.99         |
| H <sub>4</sub> Si <sub>2</sub>         | 8.36               | 8.79               | 8.21  | 8.52  | 8.19         |
| H <sub>5</sub> C <sub>2</sub>          | 8.60               | 8.59               | 8.52  | 8.56  | 8.52         |
| H <sub>4</sub> C <sub>2</sub> O        | 10.38              | 10.03              | 9.96  | 10.30 | 10.01        |
| H <sub>4</sub> C <sub>2</sub> S        | 9.15               | 8.95               | 8.92  | 8.89  | 8.91         |
| H <sub>5</sub> Si <sub>2</sub>         | 8.37               | 8.50               | 8.39  | 8.33  | 8.32         |
| H <sub>6</sub> Si <sub>2</sub>         | 10.73              | 10.44              | 10.38 | 10.14 | 10.34        |
| H <sub>4</sub> C <sub>3</sub> (cyclo)  | 10.04              | 9.67               | 9.64  | 9.12  | 9.69         |
| H <sub>4</sub> C <sub>3</sub> (allene) | 10.31              | 10.12              | 10.07 | 10.04 | 10.01        |
| 1,2,5-Thiadiazole                      | 10.10 <sup>a</sup> | 10.16              | 10.15 | 9.51  | 10.18        |
| MAE                                    |                    | 0.25               | 0.30  | 0.54  | 0.32         |
| MSE                                    |                    | -0.21              | -0.29 | -0.43 | -0.23        |

a. Reference value from the experiment reported by Pasinszki et al.<sup>15</sup>

Table 6: Comparison of vertical electron affinity (EA) values (in eV) for a set of small molecules using different methods: lrLOSC, GSC2, LOSC, and  $\Delta$ PBE. Reference values are obtained from CCSD(T)/aug-cc-pVTZ calculations.<sup>14</sup> The first EA is determined as the negative value of the lowest unoccupied molecular orbital (LUMO) energy. ‘N/A’ in the  $\Delta$ PBE column indicates convergence failure for the (N+1)-electron system in self-consistent calculations. MAE and MSE are reported for each method compared to the reference.

| Molecule          | EA    | lrLOSC (this work) | GSC2  | LOSC2 | $\Delta$ PBE |
|-------------------|-------|--------------------|-------|-------|--------------|
| HC                | 1.19  | 1.39               | 1.42  | 0.81  | 1.53         |
| H <sub>2</sub> C  | 0.83  | 0.57               | 0.72  | -0.92 | 0.37         |
| H <sub>3</sub> C  | -0.06 | -0.12              | 0.01  | -0.98 | 0.04         |
| HN                | 0.33  | 0.50               | 0.53  | -0.64 | 0.56         |
| H <sub>2</sub> N  | 0.75  | 0.75               | 0.77  | -0.33 | 0.83         |
| HO                | 1.83  | 1.86               | 1.87  | 0.47  | 1.97         |
| HSi               | 1.26  | 1.29               | 1.37  | 1.24  | N/A          |
| H <sub>2</sub> Si | 1.07  | 1.23               | 1.32  | 1.07  | 1.26         |
| H <sub>3</sub> Si | 0.93  | 0.87               | 0.97  | 0.50  | 0.96         |
| HP                | 1.02  | 1.02               | 1.10  | 0.68  | 1.07         |
| H <sub>2</sub> P  | 1.26  | 1.14               | 1.22  | 0.91  | 1.25         |
| HS                | 2.36  | 2.28               | 2.30  | 2.02  | 2.34         |
| O <sub>2</sub>    | -0.02 | -0.43              | -0.42 | 0.11  | -0.06        |
| NO                | -0.35 | -0.53              | -0.52 | 0.00  | -0.09        |
| CN                | 3.93  | 3.88               | 3.85  | 3.41  | 3.76         |
| OP                | 1.09  | 0.96               | 0.99  | 1.49  | 1.18         |
| S <sub>2</sub>    | 1.64  | 1.33               | 1.35  | 1.98  | 1.49         |
| Cl <sub>2</sub>   | 1.16  | 0.93               | 1.00  | 1.72  | 1.27         |
| C <sub>2</sub>    | 3.24  | 3.42               | 3.47  | 3.47  | 3.55         |
| C <sub>2</sub> O  | 2.18  | 1.98               | 1.99  | 2.46  | 2.10         |
| CF <sub>2</sub>   | -0.28 | -0.34              | -0.32 | -0.34 | -0.09        |
| CNO               | 3.55  | 3.29               | 3.30  | 3.80  | 3.37         |
| NO <sub>2</sub>   | 1.53  | 0.93               | 0.97  | 1.65  | 1.28         |
| O <sub>3</sub>    | 1.82  | 1.57               | 1.58  | 2.58  | 1.79         |
| OF                | 1.94  | 1.60               | 1.61  | 1.32  | 1.78         |
| O <sub>2</sub> S  | 1.06  | 0.84               | 0.86  | 1.80  | 1.02         |
| OS <sub>2</sub>   | 1.88  | 1.65               | 1.67  | 2.44  | 1.79         |

Table 7: The first EA for small molecules (continue)

| Molecule                        | EA    | lrLOSC (this work) | GSC2  | LOSC2 | $\Delta$ PBE |
|---------------------------------|-------|--------------------|-------|-------|--------------|
| HC <sub>2</sub>                 | 2.95  | 2.95               | 2.91  | 1.65  | 2.95         |
| H <sub>3</sub> C <sub>2</sub>   | 0.19  | 0.25               | 0.30  | -0.69 | 0.25         |
| H <sub>2</sub> C <sub>3</sub>   | 1.70  | 1.76               | 1.78  | 2.27  | 1.85         |
| H <sub>3</sub> C <sub>3</sub>   | 0.68  | 0.63               | 0.66  | 0.84  | 0.73         |
| HCO                             | -0.07 | -0.40              | -0.34 | -0.21 | -0.01        |
| HCF                             | 0.24  | 0.34               | 0.37  | 0.07  | 0.51         |
| CH <sub>3</sub> O               | 1.43  | 1.31               | 1.34  | 0.50  | 1.42         |
| H <sub>3</sub> CS               | 1.88  | -0.40              | -0.34 | -0.64 | -0.19        |
| H <sub>2</sub> CS               | 0.31  | 0.25               | 0.30  | 0.70  | 0.45         |
| CH <sub>2</sub> CN              | 1.54  | 1.50               | 1.51  | 1.66  | 1.54         |
| CH <sub>2</sub> NC              | 0.99  | 1.05               | 1.07  | 1.06  | 1.10         |
| HC <sub>2</sub> O               | 2.28  | 2.05               | 2.07  | 2.45  | 2.16         |
| CH <sub>2</sub> CHO             | 1.71  | 1.67               | 1.68  | 1.89  | 1.75         |
| CH <sub>3</sub> CO              | 0.16  | -0.36              | -0.23 | -0.53 | 0.31         |
| HNO                             | -0.07 | 0.11               | 0.09  | -0.26 | N/A          |
| HO <sub>2</sub>                 | 0.62  | -0.20              | -0.21 | -0.21 | N/A          |
| H <sub>5</sub> C <sub>3</sub>   | 0.38  | 0.36               | 0.39  | 0.58  | 0.46         |
| H <sub>5</sub> C <sub>2</sub> O | 1.57  | 1.47               | 1.53  | 0.43  | 1.66         |
| H <sub>5</sub> C <sub>2</sub> S | 1.95  | 1.83               | 1.86  | 1.43  | 1.88         |
| MAE                             |       | 0.22               | 0.21  | 0.54  | 0.20         |
| MSE                             |       | -0.16              | -0.13 | -0.24 | -0.05        |

## Large molecules Test set (More than 8 atoms)

Most systems in the large molecules test set are organic electron acceptors, as documented by Richard et al.<sup>16</sup>. Unless specified otherwise, the reference values are obtained from the CCSD(T)/aTZ computational vertical ionization energy (IP)/EA. For all molecules in this dataset, the augmented correlation consistent triple zeta (aug-cc- pVTZ)<sup>3</sup> basis set is employed, and the aug-cc-pVTZ-RIFIT<sup>17</sup> basis set is used as the auxiliary basis for the RI approximation and the decomposition for the SMW formula.

Table 8: Comparison of vertical ionization potential (IP) values (in eV) for a set of large molecules using different methods: lrLOSC, GSC2, LOSC, and  $\Delta$ PBE. Reference values are obtained from CCSD(T)/aug-cc-pVTZ calculations<sup>16</sup> unless specified otherwise. The first IP is determined as the negative value of the highest occupied molecular orbital (HOMO) energy. Footnotes provide details on cases where experimental or lower-level computational data were used as reference values. MAE and MSE are reported for each method compared to the reference.

| Molecule                         | Ref                | lrLOSC | GSC2  | LOSC  | $\Delta$ PBE |
|----------------------------------|--------------------|--------|-------|-------|--------------|
| Acridine                         | 7.87 <sup>a</sup>  | 7.86   | 7.45  | 7.90  | 7.58         |
| Anthracene                       | 7.47               | 7.47   | 6.99  | 7.64  | 7.10         |
| Azulene                          | 7.49               | 7.54   | 7.38  | 7.48  | 7.41         |
| Benzonitrile                     | 9.88               | 9.83   | 9.53  | 9.73  | 9.56         |
| Benzoquinone                     | 10.17              | 9.87   | 9.23  | 11.03 | 9.26         |
| Benzothiadiazole                 | 8.99 <sup>b</sup>  | 8.89   | 8.76  | 8.56  | 8.79         |
| Benzothiazole                    | 8.72 <sup>c</sup>  | 8.83   | 6.72  | 8.76  | 8.55         |
| Dichlone                         | 9.89               | 9.43   | 8.86  | 11.25 | 9.15         |
| Dinitrobenzonitrile              | 11.07              | 11.03  | 10.35 | 13.00 | 10.50        |
| Fluorene                         | 7.88 <sup>d</sup>  | 7.94   | 7.62  | 7.84  | 7.69         |
| Fumaronitrile                    | 11.40              | 11.28  | 10.81 | 11.36 | 10.84        |
| Maleicanhydride                  | 11.23              | 11.02  | 10.40 | 11.97 | 10.44        |
| NDCA                             | 8.96 <sup>a</sup>  | 9.04   | 7.69  | 9.23  | 8.77         |
| Naphthalenedione                 | 9.79               | 9.50   | 8.77  | 10.80 | 8.82         |
| Nitrobenzene                     | 10.14              | 9.97   | 9.93  | 12.10 | 9.86         |
| Nitrobenzonitrile                | 10.55              | 10.52  | 10.17 | 12.58 | 10.42        |
| Phenazine                        | 8.42               | 8.33   | 7.93  | 10.45 | 7.96         |
| Phthalicanhydride                | 10.48              | 10.33  | 9.88  | 11.73 | 10.25        |
| Phthalimide                      | 10.02              | 9.78   | 9.26  | 11.10 | 9.27         |
| TCNE                             | 11.90              | 12.05  | 11.16 | 12.65 | 11.20        |
| TCNQ                             | 9.49               | 9.11   | 9.07  | 9.30  | 9.11         |
| Tetrachloro-isobenzofuranedione  | 9.84 <sup>a</sup>  | 10.04  | 9.19  | 10.14 | 9.62         |
| Tetrachlorobenzoquinone          | 10.12              | 9.77   | 9.28  | 9.40  | 9.36         |
| Tetrafluorobenzenedicarbonitrile | 10.66              | 10.76  | 10.11 | 9.44  | 10.16        |
| Tetrafluorobenzoquinone          | 11.04              | 10.54  | 10.17 | 10.00 | 10.23        |
| 1,2,5-Thiadiazole                | 10.10 <sup>e</sup> | 10.16  | 10.15 | 9.51  | 10.18        |
| mDCBN                            | 10.37              | 10.36  | 9.88  | 10.27 | 9.90         |
| Thiophene                        | 8.86 <sup>c</sup>  | 8.83   | 8.83  | 8.44  | 9.30         |

Table 9: Comparison of vertical ionization potential (IP) values (in eV) for a set of large organic molecules using different methods: lrLOSC, GSC2, LOSC, and  $\Delta$ PBE. Reference values are obtained from CCSD(T)/aug-cc-pVTZ calculations<sup>16</sup> unless specified otherwise. The first IP is determined as the negative value of the highest occupied molecular orbital (HOMO) energy. Footnotes provide details on cases where experimental or lower-level computational data were used as reference values. MAE and MSE are reported for each method compared to the reference. (Continue)

| Molecule                        | Ref                | lrLOSC | GSC2  | LOSC  | $\Delta$ PBE |
|---------------------------------|--------------------|--------|-------|-------|--------------|
| H <sub>6</sub> C <sub>2</sub> O | 10.89 <sup>e</sup> | 10.47  | 10.32 | 10.87 | 10.17        |
| H <sub>7</sub> C <sub>3</sub>   | 7.80 <sup>e</sup>  | 7.73   | 7.65  | 7.76  | 7.61         |
| H <sub>4</sub> C <sub>4</sub> O | 9.09 <sup>e</sup>  | 8.89   | 8.87  | 8.40  | 8.89         |
| H <sub>5</sub> C <sub>4</sub> N | 8.42 <sup>e</sup>  | 8.35   | 8.26  | 8.04  | 8.28         |
| MAE                             |                    | 0.17   | 0.59  | 0.69  | 0.44         |
| MSE                             |                    | -0.12  | -0.59 | 0.33  | -0.44        |

- a. CCSD(T)/aTZ computation was not performed. Reference values are CCSD(T)/aDZ from the same literature.
- b. Reference value from experiment reported by Clark et al.<sup>18</sup>
- c. Reference value from experiment reported by Eland<sup>19</sup>
- d. Reference value from experiment reported by Meot-Ner<sup>20</sup>
- e. Large molecule in G2/97 test set.<sup>13</sup> Reference values are obtained from CCSD(T) calculations, extrapolated to the complete basis set limit as detailed in Ref Su et al.<sup>14</sup>.

Table 10: Comparison of vertical electron affinity (EA) values (in eV) for a set of large organic molecules using different methods: lrLOSC, GSC2, LOSC, and  $\Delta$ PBE. Reference values are obtained from CCSD(T)/aug-cc-pVTZ calculations<sup>16</sup> unless specified otherwise. The first EA is determined as the negative value of the lowest unoccupied molecular orbital (LUMO) energy. ‘N/A’ in the  $\Delta$ PBE column indicates convergence failure for the (N+1)-electron system in self-consistent calculations. Footnotes provide details on cases where experimental or lower-level computational data were used as reference values. MAE and MSE are reported for each method compared to the reference.

| Molecules                        | Ref   | lrLOSC | GSC2  | LOSC2 | $\Delta$ PBE |
|----------------------------------|-------|--------|-------|-------|--------------|
| Acridine                         | 0.48  | 0.81   | 0.93  | 0.83  | 0.90         |
| Anthracene                       | 0.26  | 0.40   | 0.74  | 0.57  | 0.70         |
| Azulene                          | 0.48  | 0.47   | 0.52  | 0.90  | 0.57         |
| Benzonitrile                     | -0.29 | -0.12  | -0.04 | 0.56  | N/A          |
| Benzoquinone                     | 1.46  | 1.79   | 1.80  | 2.72  | 1.83         |
| Dichlone                         | 1.82  | 2.00   | 2.31  | 2.51  | 2.12         |
| Dinitrobenzonitrile              | 1.67  | 1.49   | 2.28  | 1.64  | 2.30         |
| Fumaronitrile                    | 0.89  | 1.13   | 1.20  | 1.77  | 1.25         |
| Maleicanhydride                  | 0.92  | 1.16   | 1.18  | 1.97  | 1.23         |
| NDCA                             | 1.04  | 1.29   | 1.99  | 1.64  | 1.51         |
| Naphthalenedione                 | 1.39  | 1.61   | 1.71  | 2.20  | 1.75         |
| Nitrobenzene                     | 0.44  | 0.28   | 0.64  | 0.45  | 0.79         |
| Nitrobenzonitrile                | 1.20  | 1.16   | 1.56  | 1.35  | 1.67         |
| Phenazine                        | 1.03  | 0.94   | 1.20  | 1.32  | 1.27         |
| Phthalicanhydride                | 0.78  | 0.92   | 1.08  | 1.39  | 1.11         |
| Phthalimide                      | 0.54  | 0.66   | 0.80  | 1.27  | 0.85         |
| TCNE                             | 2.94  | 3.15   | 3.19  | 3.71  | 3.22         |
| TCNQ                             | 3.23  | 3.50   | 3.47  | 3.35  | 3.48         |
| Tetrachloro-isobenzofuranedione  | 1.41  | 1.61   | 1.81  | 1.80  | 1.81         |
| Tetrachlorobenzoquinone          | 2.36  | 2.47   | 2.60  | 3.06  | 2.62         |
| Tetrafluorobenzenedicarbonitrile | 1.51  | 1.30   | 1.70  | 2.25  | 1.72         |
| Tetrafluorobenzoquinone          | 2.18  | 2.34   | 2.37  | 3.31  | 2.38         |
| mDCBN                            | 0.54  | 0.75   | 0.86  | 1.34  | 0.89         |
| MAE                              |       | 0.18   | 0.33  | 0.59  | 0.34         |
| MSE                              |       | 0.12   | 0.33  | 0.59  | 0.34         |

## Polymers IP calculation

This section focuses on the all-trans-polyacetylene carbon chain systems.  $\text{H}(\text{HC}=\text{CH})_n\text{H}$ . The longest chain has an  $n$  value of 10, and consists of 42 atoms. Due to the absence of a well-defined LUMO in some smaller systems within this data set, only IP calculations are presented in the subsequent text. The reference IP values are derived from RAS-PT2 (max=4) computational results as reported by Shahi et al.<sup>21</sup>. In the polymer calculation, the correlation consistent triple zeta (cc-pVTZ)<sup>3</sup> basis set is employed, and the cc-pVTZ-RIFIT<sup>17</sup> basis set is used as the auxiliary basis for the RI approximation and the decomposition for the SMW formula.

# Ionization Potential for Polyacetylene

| $\text{H}(\text{HC}=\text{CH})_n\text{H}$ | Reference (RASPT2) | lrLOSC | GSC2  | LOSC2 | CASSCF | Exp       |
|-------------------------------------------|--------------------|--------|-------|-------|--------|-----------|
| 1                                         | 10.48              | 10.65  | 10.66 | 10.45 | 10.48  | 10.51     |
| 2                                         | 9.18               | 9.27   | 8.89  | 9.42  | 9.18   | 9.07      |
| 3                                         | 8.18               | 8.46   | 7.98  | 8.80  | 8.18   | 8.29-8.45 |
| 4                                         | 7.69               | 7.96   | 7.39  | 8.14  | 7.68   | 7.8-8.1   |
| 5                                         | 7.33               | 7.43   | 6.98  | 7.98  | 7.31   | N/A       |
| 6                                         | 7.04               | 7.21   | 6.66  | 7.68  | 7.04   | N/A       |
| 7                                         | 6.85               | 6.95   | 6.42  | 7.43  | 6.87   | N/A       |
| 8                                         | 6.66               | 6.86   | 6.23  | 7.41  | N/A    | N/A       |
| 9                                         | 6.56               | 6.59   | 6.06  | 7.22  | N/A    | N/A       |
| 10                                        | 6.41               | 6.52   | 5.90  | 7.17  | N/A    | N/A       |
| MAE                                       |                    | 0.15   | 0.36  | 0.54  |        |           |
| MSE                                       |                    | 0.15   | -0.32 | 0.58  |        |           |
| Infinity Extrapolation                    | 4.56               | 4.67   | 3.79  | 5.65  | 4.69   |           |

Table 11: Vertical IP (in eV) for polyacetylene chains  $\text{H}(\text{HC}=\text{CH})_n\text{H}$  with increasing chain length ( $n$ ). The IP values are compared across multiple methods: lrLOSC, GSC2, LOSC2. Reference values are obtained from RASPT2 calculations,<sup>21</sup> while experimental values (Exp) and CASSCF computational values are provided when available.<sup>21</sup> MAE and MSE are calculated with respect to the reference RASPT2 values. The "Infinity Extrapolation" values are obtained from linear regression of the IP values against  $1/\sqrt{n}$ ,<sup>14</sup> predicting the asymptotic behavior for an infinitely long polyacetylene chain. 'N/A' indicates data is unavailable for the corresponding method or chain length.

## Gas phase transition metal monoxide

Transition metal systems often present significant challenges for the  $\Delta$ SCF method due to their complex electronic structures. In this section, we compare the performance of lrLOSC with GSC2 and LOSC2, using PBE as the parent DFT functional. All molecules are modeled as diatomic systems in the gas phase, with bond lengths fixed to their experimentally determined values obtained from the work by Gutsev et al.<sup>22</sup>.

To minimize relativistic effects, the data set includes only fourth-period transition metals, as lrLOSC does not account for spin-orbit coupling. All calculations are performed using the def2-QZVPD basis set,<sup>23</sup> and the curvature matrices are evaluated explicitly without employing the RI approximation and the SMW formula.

The reference values for the gas-phase transition metal monoxide are the experimental values, with specific references provided in the corresponding table.

# Gas-phase Transition Metal Monoxide IP

| Molecules | Bond length (Å) | Exp.               | lrLOSC | GSC2  | LOSC2 |
|-----------|-----------------|--------------------|--------|-------|-------|
| CoO       | 1.629           | 8.69 <sup>24</sup> | 8.00   | 8.00  | 9.19  |
| CrO       | 1.615           | 7.85 <sup>24</sup> | 7.97   | 7.93  | 7.94  |
| CuO       | 1.724           | 9.41 <sup>25</sup> | 9.17   | 9.14  | 10.00 |
| FeO       | 1.616           | 8.56 <sup>25</sup> | 8.60   | 8.60  | 9.02  |
| MnO       | 1.648           | 8.70 <sup>24</sup> | 8.83   | 8.80  | 8.69  |
| NiO       | 1.627           | 8.77 <sup>24</sup> | 9.03   | 8.95  | 9.50  |
| ScO       | 1.668           | 6.60 <sup>24</sup> | 7.01   | 6.41  | 7.03  |
| TiO       | 1.620           | 6.82 <sup>24</sup> | 6.94   | 6.89  | 6.68  |
| VO        | 1.589           | 7.24 <sup>24</sup> | 7.41   | 7.33  | 7.12  |
| ZnO       | 1.724           | 9.34 <sup>26</sup> | 9.20   | 9.18  | 11.13 |
| MAE       |                 |                    | 0.23   | 0.19  | 0.48  |
| MSE       |                 |                    | 0.02   | -0.08 | 0.43  |

Table 12: Vertical IP (in eV) for transition metal monoxide. The IP values are compared across multiple methods: lrLOSC, GSC2, LOSC2. Reference values are obtained from experimental values. MAE and MSE are calculated with respect to the experimental values.

# Gas-phase Transition Metal Monoxide EA

| Molecule | Bond length (Å) | Exp                | lrLOSC | GSC2  | LOSC2 |
|----------|-----------------|--------------------|--------|-------|-------|
| CoO      | 1.629           | 1.45 <sup>22</sup> | 1.61   | 1.71  | 1.07  |
| CrO      | 1.615           | 1.22 <sup>27</sup> | 0.72   | 1.30  | 0.43  |
| CuO      | 1.724           | 1.78 <sup>28</sup> | 1.62   | 1.61  | 1.16  |
| FeO      | 1.616           | 1.49 <sup>29</sup> | 0.88   | 1.07  | 0.91  |
| MnO      | 1.648           | 1.38 <sup>30</sup> | 0.64   | 0.70  | 0.83  |
| NiO      | 1.627           | 1.46 <sup>31</sup> | 1.12   | 1.18  | 0.95  |
| ScO      | 1.668           | 1.35 <sup>22</sup> | 1.71   | 1.52  | -0.05 |
| TiO      | 1.620           | 1.2 <sup>32</sup>  | 1.12   | 1.52  | 0.28  |
| VO       | 1.589           | 1.23 <sup>33</sup> | 1.69   | 1.51  | -0.47 |
| ZnO      | 1.724           | 2.08 <sup>34</sup> | 2.00   | 2.04  | 2.30  |
| MAE      |                 |                    | 0.35   | 0.27  | 0.77  |
| MSE      |                 |                    | -0.15  | -0.04 | -0.72 |

Table 13: Vertical EA (in eV) for transition metal monoxide. The EA values are compared across multiple methods: lrLOSC, GSC2, LOSC2. Reference values are obtained from experimental values. MAE and MSE are calculated with respect to the experimental values.

The Delocalization Error affects not just the orbital energy but also the total energy. In the following discussion, we provide the IP energy for 18 large molecules derived from the lrLOSC corrected HOMO energy ( $\epsilon_{\text{HOMO}}^{\text{Neutral}}$ ), and compare it with the total energy difference between neutral and cation systems before and after applying lrLOSC corrections. The reference IP used is the same as the value in Table 6, and both MAE and MSE are calculated in relation to these reference values.

Table 14: Comparison of IP for 27 large molecules derived from lrLOSC corrected HOMO energies ( $\epsilon_{\text{HOMO}}^{\text{Neutral}}$ ), and total energy differences before ( $\Delta\text{PBE}$ ) and after ( $\Delta\text{lrLOSC-PBE}$ ) applying lrLOSC total energy corrections. Reference values are taken from Table 6.

| Molecule                         | Ref   | $\epsilon_{\text{HOMO}}^{\text{Neutral}}$ | $\Delta\text{PBE}$ | $\Delta\text{lrLOSC-PBE}$ |
|----------------------------------|-------|-------------------------------------------|--------------------|---------------------------|
| Acridine                         | 7.87  | 7.86                                      | 7.58               | 7.71                      |
| Anthracene                       | 7.47  | 7.47                                      | 7.10               | 7.35                      |
| Azulene                          | 7.49  | 7.54                                      | 7.41               | 7.47                      |
| Benzonitrile                     | 9.88  | 9.83                                      | 9.56               | 9.80                      |
| Benzoquinone                     | 10.17 | 9.87                                      | 9.26               | 9.37                      |
| Benzothiadiazole                 | 8.99  | 8.89                                      | 8.79               | 8.85                      |
| Benzothiazole                    | 8.72  | 8.83                                      | 8.55               | 8.71                      |
| Dichlone                         | 9.89  | 9.43                                      | 9.15               | 9.77                      |
| Dinitrobenzonitrile              | 11.07 | 11.03                                     | 10.50              | 10.90                     |
| Fluorene                         | 7.88  | 7.94                                      | 7.69               | 7.91                      |
| Fumaronitrile                    | 11.40 | 11.28                                     | 10.84              | 11.26                     |
| Maleicanhydride                  | 11.23 | 11.02                                     | 10.44              | 10.61                     |
| NDCA                             | 8.96  | 9.04                                      | 8.77               | 8.98                      |
| Naphthalenedione                 | 9.79  | 9.50                                      | 8.82               | 9.01                      |
| Nitrobenzene                     | 10.14 | 9.97                                      | 9.86               | 9.87                      |
| Phenazine                        | 8.42  | 8.33                                      | 7.96               | 7.98                      |
| Nitrobenzonitrile                | 10.55 | 10.52                                     | 10.42              | 10.47                     |
| Phthalicanhydride                | 10.48 | 10.33                                     | 10.25              | 10.25                     |
| Phthalimide                      | 10.02 | 9.78                                      | 9.27               | 9.50                      |
| TCNE                             | 11.90 | 12.05                                     | 11.20              | 11.59                     |
| TCNQ                             | 9.49  | 9.11                                      | 9.11               | 9.21                      |
| Tetrachloro-isobenzofuranedione  | 9.87  | 10.04                                     | 9.62               | 10.14                     |
| Tetrachlorobenzoquinone          | 10.12 | 9.77                                      | 9.36               | 9.45                      |
| Tetrafluorobenzenedicarbonitrile | 10.66 | 10.03                                     | 10.16              | 10.20                     |
| Tetrafluorobenzoquinone          | 11.04 | 10.54                                     | 10.23              | 10.35                     |
| mDCBN                            | 10.37 | 10.27                                     | 9.90               | 10.14                     |
| Thiophene                        | 8.86  | 8.83                                      | 9.30               | 9.30                      |
| MAE                              |       | 0.16                                      | 0.44               | 0.30                      |
| MSE                              |       | -0.11                                     | -0.43              | -0.24                     |

## References

- (1) William H. Press; Brian P.P. Flannery; Saul A. Teukolsky; William T. Vetterling *Numerical Recipes in C: The Art of Scientific Computing*; Cambridge University Press: New York, 1988; pp 72–81.
- (2) Ren, X.; Rinke, P.; Blum, V.; Wieferink, J.; Tkatchenko, A.; Sanfilippo, A.; Reuter, K.; Scheffler, M. Resolution-of-identity approach to Hartree-Fock, hybrid density functionals, RPA, MP2 and GW with numeric atom-centered orbital basis functions. *New J. Phys.* **2012**, *14*, 053020, arXiv: 1201.0655.
- (3) Dunning, T. H. Gaussian basis sets for use in correlated molecular calculations. I. The atoms boron through neon and hydrogen. *J. Chem. Phys.* **1989**, *90*, 1007–1023.
- (4) Hättig, C. Optimization of Auxiliary Basis Sets for RI-MP2 and RI-CC2 Calculations: Core-Valence and Quintuple- $\zeta$  Basis Sets for H to Ar and QZVPP Basis Sets for Li to Kr. *Phys. Chem. Chem. Phys.* **2005**, *7*, 59–66.
- (5) Li, C.; Yang, W. On the piecewise convex or concave nature of ground state energy as a function of fractional number of electrons for approximate density functionals. *J. Chem. Phys.* **2017**, *146*, 074107.
- (6) Kohn, W.; Sham, L. J. Self-Consistent Equations Including Exchange and Correlation Effects. *Phys. Rev. A* **1965**, *140*, 1133–1138.
- (7) Mei, Y.; Chen, Z.; Yang, W. Exact second-order corrections and accurate quasiparticle energy calculations in density functional theory. *J. Phys. Chem. Lett.* **2021**, *12*, 7236–7244.
- (8) Frisch, M. J. et al. Gaussian~16 Revision C.01. 2016.
- (9) [Http://www.qm4d.info](http://www.qm4d.info) QM4D. <http://www.qm4d.info>.

- (10) Perdew, J. P.; Burke, K.; Ernzerhof, M. Generalized Gradient Approximation Made Simple. *Phys. Rev. Lett.* **1996**, *77*, 3865–3868.
- (11) Gilbert, A. T. B.; Besley, N. A.; Gill, P. M. W. Self-consistent field calculations of excited states using the maximum overlap method (MOM). *J. Phys. Chem. A* **2008**, *112*, 13164–13171.
- (12) Sun, Q.; Berkelbach, T. C.; Blunt, N. S.; Booth, G. H.; Guo, S.; Li, Z.; Liu, J.; McClain, J. D.; Sayfutyarova, E. R.; Sharma, S.; Wouters, S.; Chan, G. K. L. PySCF: the Python-based simulations of chemistry framework. *Wiley Interdiscip Rev. Comput Mol Sci* **2018**, *8*, e1340.
- (13) Curtiss, L. A.; Raghavachari, K.; Redfern, P. C.; Pople, J. A. Assessment of Gaussian-2 and density functional theories for the computation of enthalpies of formation. *J. Chem. Phys.* **1997**, *106*, 1063–1079.
- (14) Su, N. Q.; Mahler, A.; Yang, W. Preserving Symmetry and Degeneracy in the Localized Orbital Scaling Correction Approach. *J. Phys. Chem. Lett.* **2020**, *11*, 1528–1535.
- (15) Pasinszki, T.; Krebsz, M.; Vass, G. Ground and ionic states of 1,2,5-thiadiazoles: An UV-photoelectron spectroscopic and theoretical study. *J. Mol Struct* **2010**, *966*, 85–91.
- (16) Richard, R. M.; Marshall, M. S.; Dolgounitcheva, O.; Ortiz, J. V.; Brédas, J. L.; Marom, N.; Sherrill, C. D. Accurate Ionization Potentials and Electron Affinities of Acceptor Molecules I. Reference Data at the CCSD(T) Complete Basis Set Limit. *J. Chem. Theory Comput.* **2016**, *12*, 595–604.
- (17) Weigend, F.; Köhn, A.; Hättig, C.; Kö, A.; Karlsruhe, F. Efficient use of the correlation consistent basis sets in resolution of the identity MP2 calculations (Christof Hättig a). *J. Chem. Phys.* **2002**, *116*, 3175–3183.

- (18) Clark, P. A.; Gleiter, R.; Heilbronner, E. Photoelectron spectra of planar sulfur heterocycles. *Tetrahedron* **1973**, *29*, 3085–3089.
- (19) Eland, J. H. D. Photoelectron spectra of conjugated hydrocarbons and heteromolecules. *Int J. Mass Spectrom Ion Phys.* **1969**, *2*, 471–484.
- (20) Meot-Ner, M. Ion thermochemistry of low-volatility compounds in the gas phase. 3. Polycyclic aromatics: Ionization energies, proton and hydrogen affinities. Extrapolations to graphite. *J. Phys. Chem.* **1980**, *84*, 2716–2723.
- (21) Shahi, A. R. M.; Cramer, C. J.; Gagliardi, L. Second-order perturbation theory with complete and restricted active space reference functions applied to oligomeric unsaturated hydrocarbons. *Phys. Chem. Chem. Phys.* **2009**, *11*, 10964–10972.
- (22) Gutsev, G. L.; Andrews, L.; Bauschlicher, J. Similarities and Differences in the Structure of 3d-Metal Monocarbides and Monoxides. *Theor. Chem. Acc.* **2003**, *109*, 298–308.
- (23) Weigend, F.; Ahlrichs, R. Balanced basis sets of split valence, triple zeta valence and quadruple zeta valence quality for H to Rn: Design and assessment of accuracy. *Phys. Chem. Chem. Phys.* **2005**, *7*, 3297–3305.
- (24) Fisher, E. R.; Elkind, J. L.; Clemmer, D. E.; Georgiadis, R.; Loh, S. K.; Aristov, N.; Sunderlin, L. S.; Armentrout, P. B. Reactions of Fourth-Period Metal Ions (Ca<sup>+</sup>-Zn<sup>+</sup>) with O<sub>2</sub>: Metal-oxide Ion Bond Energies. *J. Chem. Phys.* **1990**, *93*, 2676–2691.
- (25) Metz, R. B.; Nicolas, C.; Ahmed, M.; Leone, S. R. Direct Determination of the Ionization Energies of FeO and CuO with VUV Radiation. *J. Chem. Phys.* **2005**, *123*, 114313.
- (26) Clemmer, D. E.; Dalleska, N. F.; Armentrout, P. B. Reaction of Zn<sup>+</sup> with NO<sub>2</sub>. The Gas-Phase Thermochemistry of ZnO. *J. Chem. Phys.* **1991**, *95*, 7263–7268.

- (27) Wenthold, P. G.; Gunion, R. F.; Lineberger, W. C. Ultraviolet Negative-Ion Photoelectron Spectroscopy of the Chromium Oxide Negative Ion. *Chem. Phys. Lett.* **1996**, *258*, 101–106.
- (28) Polak, M. L.; Gilles, M. K.; Ho, J.; Lineberger, W. C. Photoelectron Spectroscopy of Copper Oxide (CuO<sup>-</sup>). *J. Phys. Chem.* **1991**, *95*, 3460–3463.
- (29) Engelking, P. C.; Lineberger, W. C. Laser Photoelectron Spectrometry of FeO<sup>-</sup>: Electron Affinity, Electronic State Separations, and Ground State Vibrations of Iron Oxide, and a New Ground State Assignment. *J. Chem. Phys.* **1977**, *66*, 5054–5058.
- (30) Gutsev, G. L.; Rao, B. K.; Jena, P.; Li, X.; Wang, L.-S. Experimental and Theoretical Study of the Photoelectron Spectra of MnO<sub>x</sub> (X=1–3) Clusters. *J. Chem. Phys.* **2000**, *113*, 1473–1483.
- (31) Wu, H.; Wang, L.-S. A Study of Nickel Monoxide (NiO), Nickel Dioxide (ONiO), and Ni(O<sub>2</sub>) Complex by Anion Photoelectron Spectroscopy. *J. Chem. Phys.* **1997**, *107*, 16–21.
- (32) Wu, H.; Wang, L.-S. Electronic Structure of Titanium Oxide Clusters: TiO<sub>y</sub> (y = 1–3) and (TiO<sub>2</sub>)<sub>n</sub> (n = 1–4). *J. Chem. Phys.* **1997**, *107*, 8221–8228.
- (33) Wu, H.; Wang, L.-S. A Photoelectron Spectroscopic Study of Monovanadium Oxide Anions (VO<sub>x</sub><sup>-</sup>, X=1–4). *J. Chem. Phys.* **1998**, *108*, 5310–5318.
- (34) Fancher, C. A.; de Clercq, H. L.; Thomas, O. C.; Robinson, D. W.; Bowen, K. H. Zinc Oxide and Its Anion: A Negative Ion Photoelectron Spectroscopic Study. *J. Chem. Phys.* **1998**, *109*, 8426–8429.
